# Supplementary material for: Polylogarithmic-depth controlled-NOT gates without ancilla qubits
Source: arXiv:2312.13206 ancillary file (2024-06-07)
Supplement: Supplementary file 1 [file supplementary_information.pdf]

# Supplementary Information for: Polylogarithmic-depth controlled-NOT gates without ancilla qubits

Baptiste Claudon,<sup>1,2,\*</sup> Julien Zylberman,<sup>3</sup> César Feniou,<sup>1,2</sup> Fabrice  
Debbasch,<sup>3</sup> Alberto Peruzzo,<sup>1</sup> and Jean-Philip Piquemal<sup>1,2,†</sup>

<sup>1</sup>*Qubit Pharmaceuticals, Advanced Research Department, 75014 Paris, France*

<sup>2</sup>*Sorbonne Université, LCT, UMR 7616 CNRS, 75005 Paris, France*

<sup>3</sup>*Sorbonne Université, Observatoire de Paris, Université PSL, CNRS, LERMA, 75005 Paris, France*

## SUPPLEMENTARY NOTE 1 - STEP BY STEP STUDY OF THE PROPOSED QUANTUM CIRCUITS

**Further notations.** Before proving the correctness of the method, further notations need to be introduced. The operator  $\oplus : \{0, 1\}^2 \rightarrow \{0, 1\}$  is used to denote addition modulo 2, while  $\boxplus : \cup_{n=1}^{\infty} \{0, 1\}^n \times \{0, 1\}^n \rightarrow \cup_{n=1}^{\infty} \{0, 1\}^n$  signifies bitwise addition modulo two:  $(x_1, \dots, x_n) \boxplus (y_1, \dots, y_n) = (x_1 \oplus y_1, \dots, x_n \oplus y_n)$ . Let  $c : \cup_{n=1}^{\infty} \{0, 1\}^n \rightarrow \{0, 1\}$ ,  $(x_1, \dots, x_n) \mapsto \prod_{j=1}^n x_j$ . Also, let  $\bar{c} : \cup_{n=1}^{\infty} \{0, 1\}^n \rightarrow \{0, 1\}$ ,  $(x_1, \dots, x_n) \mapsto \prod_{j=1}^n (1 - x_j)$ . It will be practical to denote with the same symbol  $R$  a set of qubits and the bistring associated with a computational basis state label in the  $|\cdot\rangle$  notation. The operations  $c$  and  $\bar{c}$  will turn out to be very useful since for any multi-qubit register  $R$ , target qubit register  $t$  and one of their computational basis states  $|R, t\rangle$ :  $\mathcal{C}_R^t |R, t\rangle = |R, t \oplus c(R)\rangle$  and  $\mathcal{C}_R^t = |R, t \oplus \bar{c}(R)\rangle$ . For an ancilla qubit  $a$ , it also holds that  $\mathcal{C}_{R \cup a}^t |R, a, t\rangle = |R, a, t \oplus c(a)\bar{c}(R)\rangle$ .

Let  $n > 4$  and  $p = \lfloor \sqrt{n} \rfloor$ . Again, write  $R = \{q_j\}_{j=0}^{n-1}$ . Let  $R \supset R_0 = \{q_i\}_{i=0}^{2p-1}$  be a first subregister of  $2p$  control qubits, and for each  $i \geq 1$ , let  $R \supset R_i = \{q_j \text{ if } j \leq n\}_{j=(1+i)p}^{(2+i)p-1}$  be other subregisters of size at most  $p$ . Let  $R_0^* = \{q_i \in R_0 : R_{i+1} \neq \emptyset\}$  and  $R'_0 = R_0 \setminus R_0^*$ . Finally, let  $b = |R_0^*|$ .

The analysis of the construction follows the steps given below.

- First, the zeroed-ancilla circuit is proven to be correct.
- Second, the borrowed-ancilla circuit is proven to be correct.
- Third, it is shown that each of the smaller multi-controlled NOT appearing in the borrowed-ancilla circuit can be achieved with the help of a locally borrowed ancilla.
- Fourth, the recursion characterising the circuit depth is solved.

### A. Analysis of $\mathcal{U}_0$

The single-zeroed-ancilla circuit corresponds to the unitary operation

$$\mathcal{U}_0 = \mathcal{C}_{R_0}^a \left( \prod_{i=1}^b \mathcal{C}_{R_i}^{q_{i-1}} \right) \mathcal{C}_{R_0^* \cup a}^t \left( \prod_{i=1}^b \mathcal{C}_{R_i}^{q_{i-1}} \right) \mathcal{C}_{R_0}^a = \mathcal{C}_{R_0}^a \mathfrak{C} \mathcal{C}_{R_0}^a. \quad (1)$$

Proving that  $\mathcal{U}_0$  performs the desired operation relies on the following lemma.

*Lemma 1.* It holds that:

$$c(R_0)\bar{c}(R_0^* \boxplus (c(R_1), \dots, c(R_b))) = c(R). \quad (2)$$

It can be noted that  $R_0^* \boxplus (c(R_1), \dots, c(R_b)) = (q_0 \oplus c(R_1), \dots, q_{b-1} \oplus R_b)$ .

---

\* baptiste.claudon@qubit-pharmaceuticals.com

† jean-philip.piquemal@sorbonne-universite.fr

*Proof.* Assume that  $c(R) = 1$ . Necessarily all the qubits in  $R$  are in state 1 and for each  $i \in \{0, \dots, b\}$ ,  $R_i$  verifies  $c(R_i) = 1$ . In particular, for each  $i \in \{1, \dots, b\}$ ,  $q_{i-1} \oplus c(R_i) = 1 \oplus 1 = 0$ . As a consequence,  $\bar{c}(R_0^* \boxplus (c(R_1), \dots, c(R_b))) = \bar{c}(q_0 \oplus R_1, q_1 \oplus R_2, \dots, q_{b-1} \oplus R_b) = \prod_{i=1}^b 1 = 1$ . Summarising:

$$c(R) = 1 \implies c(R_0) \bar{c}(R_0^* \boxplus (c(R_1), \dots, c(R_b))) = 1 = c(R). \quad (3)$$

Now, assume that  $c(R) = 0$ . If  $c(R_0) = 0$ , then  $c(R_0) \bar{c}(R_0^* \boxplus (c(R_1), \dots, c(R_b))) = 0 = c(R)$  and we are done. Thus, assume that  $c(R_0) = 1$ . Since  $c(R) = 0$ , there must exists a qubit  $q_k \in R \setminus R_0$  in state  $|0\rangle$ . Let  $j \in \{1, \dots, b\}$  be the register index such that  $q_k \in R_j$ . Necessarily,  $c(R_j) = 0$ . However, since  $q_{j-1} \in R_0$ ,  $q_{j-1} \oplus c(R_j) = q_{j-1} = 1$ . It follows that:

$$\bar{c}(R_0^* \boxplus (c(R_1), \dots, c(R_b))) = (1 - (q_{j-1} \oplus c(R_j))) \prod_{l=1, l \neq j}^b (1 - (q_{l-1} \oplus R_l)) = 0 \prod_{l=1, l \neq j}^b (1 - (q_{l-1} \oplus R_l)) = 0. \quad (4)$$

Summarising,

$$c(R) = 0 \implies c(R_0) \bar{c}(R_0^* \boxplus (c(R_1), \dots, c(R_b))) = 0 = c(R). \quad (5)$$

Therefore, in any case,  $c(R) = c(R_0) \bar{c}(R_0^* \boxplus (c(R_1), \dots, c(R_b)))$ .

Let us also compute the action of  $\mathfrak{C}$  on an arbitrary computational basis state  $|R_0^*, R'_0, R \setminus R_0, a, t\rangle$ .

*Lemma 2.* The following equation holds for any computational basis state  $|R_0^*, R'_0, R \setminus R_0, a, t\rangle$ .

$$\mathfrak{C} |R_0^*, R'_0, R \setminus R_0, a, t\rangle = |R_0^*, R'_0, R \setminus R_0, a, t \oplus a \bar{c}(R_0^* \boxplus (R_1, \dots, R_b))\rangle. \quad (6)$$

*Proof.*

$$\begin{aligned} \mathfrak{C} |R_0^*, R'_0, R \setminus R_0, a, t\rangle &= \left( \prod_{i=1}^b \mathcal{C}_{R_i}^{q_{i-1}} \right) \mathcal{C}_{R_0^* \cup a}^t \left( \prod_{i=1}^b \mathcal{C}_{R_i}^{q_{i-1}} \right) |R_0^*, R'_0, R \setminus R_0, a, t\rangle \\ &= \left( \prod_{i=1}^b \mathcal{C}_{R_i}^{q_{i-1}} \right) \mathcal{C}_{R_0^* \cup a}^t |R_0^* \boxplus (c(R_1), \dots, c(R_b)), R'_0, R \setminus R_0, a, t\rangle \\ &= \left( \prod_{i=1}^b \mathcal{C}_{R_i}^{q_{i-1}} \right) |R_0^* \boxplus (c(R_1), \dots, c(R_b)), R'_0, R \setminus R_0, a, t \oplus c(a) \bar{c}(R_0^* \boxplus (R_1, \dots, R_b))\rangle \\ &= |R_0^*, R'_0, R \setminus R_0, a, t \oplus c(a) \bar{c}(R_0^* \boxplus (R_1, \dots, R_b))\rangle. \end{aligned} \quad (7)$$

Conclude by noticing that for a single-qubit labelled by  $a$  in a state of the computational basis,  $a = c(a)$ .

Let us verify that for any computational basis state of the form  $|R_0^*, R'_0, R \setminus R_0, 0, t\rangle$ ,  $\mathcal{U}_0 |R_0^*, R'_0, R \setminus R_0, 0, t\rangle = \mathcal{C}_R^t |R_0^*, R'_0, R \setminus R_0, 0, t\rangle$ .

$$\begin{aligned} \mathcal{U}_0 |R_0^*, R'_0, R \setminus R_0, 0, t\rangle &= \mathcal{C}_{R_0}^a \mathfrak{C} \mathcal{C}_{R_0}^a |R_0^*, R'_0, R \setminus R_0, 0, t\rangle \\ &= \mathcal{C}_{R_0}^a \mathfrak{C} |R_0^*, R'_0, R \setminus R_0, c(R_0), t\rangle && \text{by definition of } C^n(X) \text{ and } c \\ &= \mathcal{C}_{R_0}^a |R_0^*, R'_0, R \setminus R_0, c(R_0), t \oplus c(R_0) \bar{c}(R_0^* \boxplus (R_1, \dots, R_b))\rangle && \text{by Lemma 2} \\ &= |R_0^*, R'_0, R \setminus R_0, 0, t \oplus c(R_0) \bar{c}(R_0^* \boxplus (R_1, \dots, R_b))\rangle && \text{by definition of } C^n(X) \text{ and } c \\ &= |R_0^*, R'_0, R \setminus R_0, 0, t \oplus c(R)\rangle && \text{by Lemma 1} \\ &= \mathcal{C}_R^t |R_0^*, R'_0, R \setminus R_0, 0, t\rangle. \end{aligned} \quad (8)$$

By linearity,  $\mathcal{U}_0$  performs the right operation on any superposition of the computational basis with ancilla in state  $|0\rangle$ , hence any state with zeroed ancilla.

### B. Analysis of $\mathcal{U}$

Following the same logic, the correctness of single-borrowed-ancilla circuit is proven. This circuit acts as:

$$\mathcal{U} = \left( \prod_{i=1}^b \mathcal{C}_{R_i}^{q_i-1} \right) \mathcal{C}_{R_0^* \cup a}^t \left( \prod_{i=1}^b \mathcal{C}_{R_i}^{q_i-1} \right) \mathcal{U}_0 = \mathfrak{C} \mathcal{U}_0. \quad (9)$$

The evolution of an arbitrary input state  $|R_0^*, R'_0, R \setminus R_0, a, t\rangle$  is given in equation 10.

$$\begin{aligned} \mathcal{U} |R_0^*, R'_0, R \setminus R_0, a, t\rangle &= \mathfrak{C} \mathcal{C}_{R_0}^a \mathfrak{C} \mathcal{C}_{R_0}^a |R_0^*, R'_0, R \setminus R_0, a, t\rangle \\ &= \mathfrak{C} \mathcal{C}_{R_0}^a \mathfrak{C} |R_0^*, R'_0, R \setminus R_0, a \oplus c(R_0), t\rangle \\ &= \mathfrak{C} \mathcal{C}_{R_0}^a |R_0^*, R'_0, R \setminus R_0, a \oplus c(R_0), t \oplus (a \oplus c(R_0)) \bar{c}(R_0^* \boxplus (c(R_1), \dots, c(R_b)))\rangle \quad \text{by Lemma 2} \\ &= \mathfrak{C} \mathcal{C}_{R_0}^a |R_0^*, R'_0, R \setminus R_0, a \oplus c(R_0), t \oplus c(R) \oplus a \bar{c}(R_0^* \boxplus (c(R_1), \dots, c(R_b)))\rangle \quad \text{by Lemma 1} \\ &= \mathfrak{C} |R_0^*, R'_0, R \setminus R_0, a, t \oplus c(R) \oplus a \bar{c}(R_0^* \boxplus (c(R_1), \dots, c(R_b)))\rangle \\ &= |R_0^*, R'_0, R \setminus R_0, a, t \oplus c(R) \oplus 2a \bar{c}(R_0^* \boxplus (c(R_1), \dots, c(R_b)))\rangle \quad \text{by Lemma 2} \\ &= |R_0^*, R'_0, R \setminus R_0, a, t \oplus c(R)\rangle \\ &= \mathcal{C}_R^t |R_0^*, R'_0, R \setminus R_0, a, t\rangle. \end{aligned} \quad (10)$$

By linearity,  $\mathcal{U} = \mathcal{C}_R^t$ .

### C. Each smaller multi-controlled NOT gate has a borrowed ancilla at its disposal

*Lemma 3.* The register  $R'_0$  has more qubits than the register  $R_0^*$ :  $|R'_0| \geq |R_0^*|$ .

*Proof.*  $|R \setminus R_0| = n - 2p < (p+1)^2 - 2p = p^2 + 1$ . Thus,  $|R \setminus R_0| \leq p^2$ . In words, the qubits in  $R \setminus R_0$  can be gathered in at most  $p$  subregisters of size  $p$ . In equation,  $|R_0^*| \leq p$ . Finally,  $|R'_0| = |R_0| - |R_0^*| \geq 2p - p = p \geq |R_0^*|$ .

As a consequence, each of the factors in

$$\prod_{i=1}^b \mathcal{C}_{R_i}^{q_i-1} \quad (11)$$

can be executed with the help of a borrowed ancilla in  $R'_0$ .

### D. Solving the recursion

The operation with the highest number of control qubits is controlled by the state of  $R_0$ , of size  $|R_0| = 2p$ . It is applied twice. A layer of  $C^p(X)$  gates is applied four times, and a layer of  $C^{p+1}(X)$  (or even  $C^p(X)$  in some cases) gates is applied twice. The overall depth can be uniformly bounded by the depth of eight successive  $C^{2p}(X)$  gates plus a constant term corresponding to the layers of  $X$  gates required by the white controls. Let us conclude the analysis by upper bounding the resulting depth. Let  $D(n)$  be the depth of circuit  $C^n(X)$ . Assume that  $n = 2^{k+2}$ ,

$$D(2^{k+2}) \leq 2D\left(2^{\frac{k+2}{2}+1}\right) + 4D\left(2^{\frac{k+2}{2}}\right) + 2D\left(2^{\frac{k+2}{2}} + 1\right) + 4 \leq 8D\left(2^{\frac{k+2}{2}+1}\right) + 4 = 8D\left(2^{\frac{k}{2}+2}\right) + 4 \in \mathcal{O}\left(k^{\log(8)}\right) \quad (12)$$

by the Master Theorem 1. In terms of  $n$ , the depth of the  $n$ -control gate is  $\mathcal{O}(\log(n)^3)$ .

## SUPPLEMENTARY NOTE 2 - MASTER THEOREM

The Master Theorem 1 is a fundamental theorem for the analysis of dynamical programming algorithms [1]. The master method, based on this theorem, provides asymptotic growths for recurrences of the form  $T(n) = aT(n/b) + f(n)$ , where  $a \geq 1$ ,  $b > 1$ .

*Theorem 1.* Let  $a \geq 1$  and  $b > 1$  be constants, let  $f(n)$  be a function and let  $T(n)$  be defined on the nonnegative integers by the recurrence

$$T(n) = aT(n/b) + f(n), \quad (13)$$

where we interpret  $n/b$  to mean either  $\lfloor n/b \rfloor$  or  $\lceil n/b \rceil$ . Then  $T(n)$  has the following asymptotic bounds:

1. If  $f(n) \in \mathcal{O}(n^{\log_b(a)-\epsilon})$  for some constant  $\epsilon > 0$ , then  $T(n) = \Theta(n^{\log_b(a)})$ .
2. If  $f(n) = \Theta(n^{\log_b(a)})$ , then  $T(n) = \Theta(n^{\log_b(a)} \log n)$ .
3. If  $f(n) = \Omega(n^{\log_b(a)+\epsilon})$  for some constant  $\epsilon > 0$ , and if  $af(n/b) \leq cf(n)$  for some constant  $c < 1$  and all sufficiently large  $n$ , then  $T(n) = \Theta(f(n))$ .

### SUPPLEMENTARY NOTE 3 - CIRCUIT SIZE

Let us show that the size  $S(n)$  of a  $C^n(X)$  gate is  $\tilde{\Theta}(n)$ . Clearly,  $S(n) \in \Omega(n)$ . Let us show that  $S(n) \in \mathcal{O}(n \log(n)^4)$ . Let  $n = 2^{k+2}$ . Then,

$$S(2^{k+2}) \leq 4 \left( 2^{k/2+2} S(2^{k/2+2}) + 1 \right). \quad (14)$$

Define  $\tilde{S}(n) \equiv S(n)/n$ . Then,

$$\tilde{S}(2^{k+2}) \leq 16\tilde{S}(2^{k/2+2}) + \mathcal{O}(1) \in \mathcal{O}(k^4). \quad (15)$$

As a consequence,  $S(n) \in \mathcal{O}(n \log(n)^4)$  and  $S(n) \in \tilde{\Theta}(n)$ .

---

[1] T. H. Cormen, C. E. Leiserson, R. L. Rivest, and C. Stein, Introduction to Algorithms, Third Edition, 3rd ed. (The MIT Press, 2009).
